# Supplementary material for: NAIS-Net: Stable Deep Networks from Non-Autonomous Differential Equations
Source: arXiv:1804.07209 source file (2021-05-21)
Supplement: Supplementary file 1 [file appendix5.tex]

\section{Pattern-Dependent Processing Depth}\label{sec:depth}
This section explores the
idea of having NAIS-Net implement {\em pattern-dependent processing
  depth} where the number of processing stages applied to each input
pattern is determined by the network itself. As discussed in the main paper,
 this can be done for instance when ReLU activations are used as the asymptotic
 input-output mapping is non-linear. For $\tanh$ activations, on the other hand,
 the mapping becomes linear as the number of unroll steps increase
 and we are therefore interested
 in retaining  
 the transient behaviour. This might require additional components 
 to be added to the architecture \citep[see][]{graves2016a,veit2017a,figurnov2017a}
 and
 is left for future work. 
 In the following, 
 we will therefore consider the case of ReLU activations and test our 
 claims on the 
 CIFAR-10 dataset. 

In the main paper, the number of unrolling steps per block in the
 experiments was fixed.  A more general and potentially more
powerful setup is to have the processing depth adapt automatically.
Since NAIS-Net blocks are guaranteed to converge to a pattern-dependent
steady state after an indeterminate number of iterations, processing
depth can be controlled dynamically by terminating the unrolling
process whenever the distance between a layer representation, $x(i)$,
and that of the immediately previous layer, $x(i-1)$, drops below a
specified threshold.

With this mechanism, NAIS-Net can determine the processing depth for
each input pattern.  Intuitively, one could speculate that similar
input patterns would require similar processing depth in order to be
mapped to the same region in latent space.  To explore this
hypothesis, NAIS-Net was trained on CIFAR-10 with an unrolling
threshold of $\epsilon=10^{-4}$.  At test time the network was
unrolled using the same threshold.

Figure~\ref{fig:frogplot} shows the number of iterations required over
the course of training to cross the depth threshold, $\epsilon$, for
five selected network blocks. As training progresses, depth increases
almost monotonically at different rates per block, until becoming
relatively stable.

Figure~\ref{fig:histdepth_sup} shows selected sample images from four
different classes organized according to the final network depth used
to classify them after training.  The qualitative differences seen from
low to high depth suggests that NAIS-Net is using processing depth as
an additional degree of freedom so that, for a given training run, the
network learns to use models of different complexity (depth) for
different types of inputs within each class.  To be clear, the hypothesis is not that
depth correlates to some notion of input complexity where the same images are
always classified at the same depth across runs.
\begin{figure}[t]
    \noindent\begin{minipage}{0.44\columnwidth}
    \begin{figure}[H]
 \centering
    \includegraphics[width=\columnwidth]{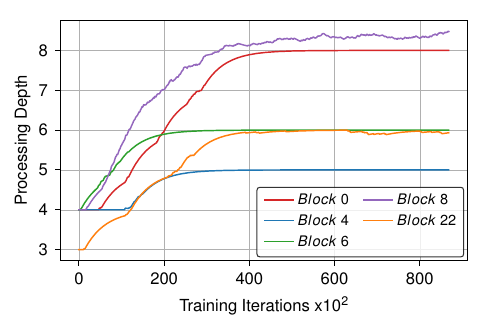}
    \caption{{\bf Processing depth for different NAIS-Net blocks during
        training.} The figure shows the number of iterations ($y$-axis), of $5$
        different blocks taken NAIS-Net at various stages of training ($x$-axis)
        for the CIFAR-10 image classification task. }
    \label{fig:maxiters}
\end{figure}
\vspace{0.6cm}
\end{minipage}~~~~~
    \noindent\begin{minipage}{0.44\columnwidth}
 \begin{figure}[H]
   \centering
     \includegraphics[width=\columnwidth]{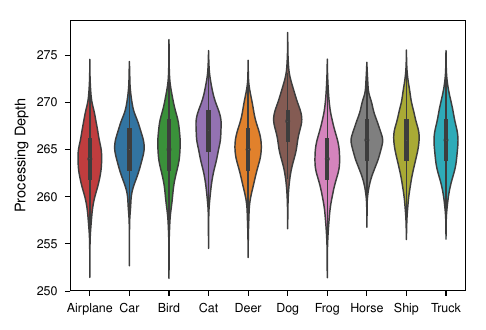}
     \caption{{\bf Final NAIS-Net depth distribution for CIFAR-10 classes.}
     Depth over the classes is statistically different. The Kruskal-Wallis
     one-way ANOVA test, under the null hypothesis of all depths coming from
     the same distribution, produced a \textit{p}-value of zero. Pair-wise testing
     resulted in statistically different depths in $86.7\%$ of cases, with a
     $95\%$ confidence level.}
     \label{fig:frogplot}
 \end{figure}
 \end{minipage}
 \end{figure} 
 
Figure~\ref{fig:frogplot} shows a violin plot of the final network
depth for each CIFAR-10 class. To highlight any statistical
differences, the null hypothesis that the network depth being drawn
from the same distribution for all classes was tested first.  One-way
ANOVA test~\cite{kruskal1952} was performed over all the classes
resulting in a \textit{p}-value of zero, thus fully rejecting the null
hypothesis.  The same test was performed on each pair of classes: the
$86.7\%$ of depth distributions is statistically different with $95\%$
confidence.

\begin{figure}[t]
  \centering
   \subfigure[frog]{\includegraphics[width=0.49\textwidth]{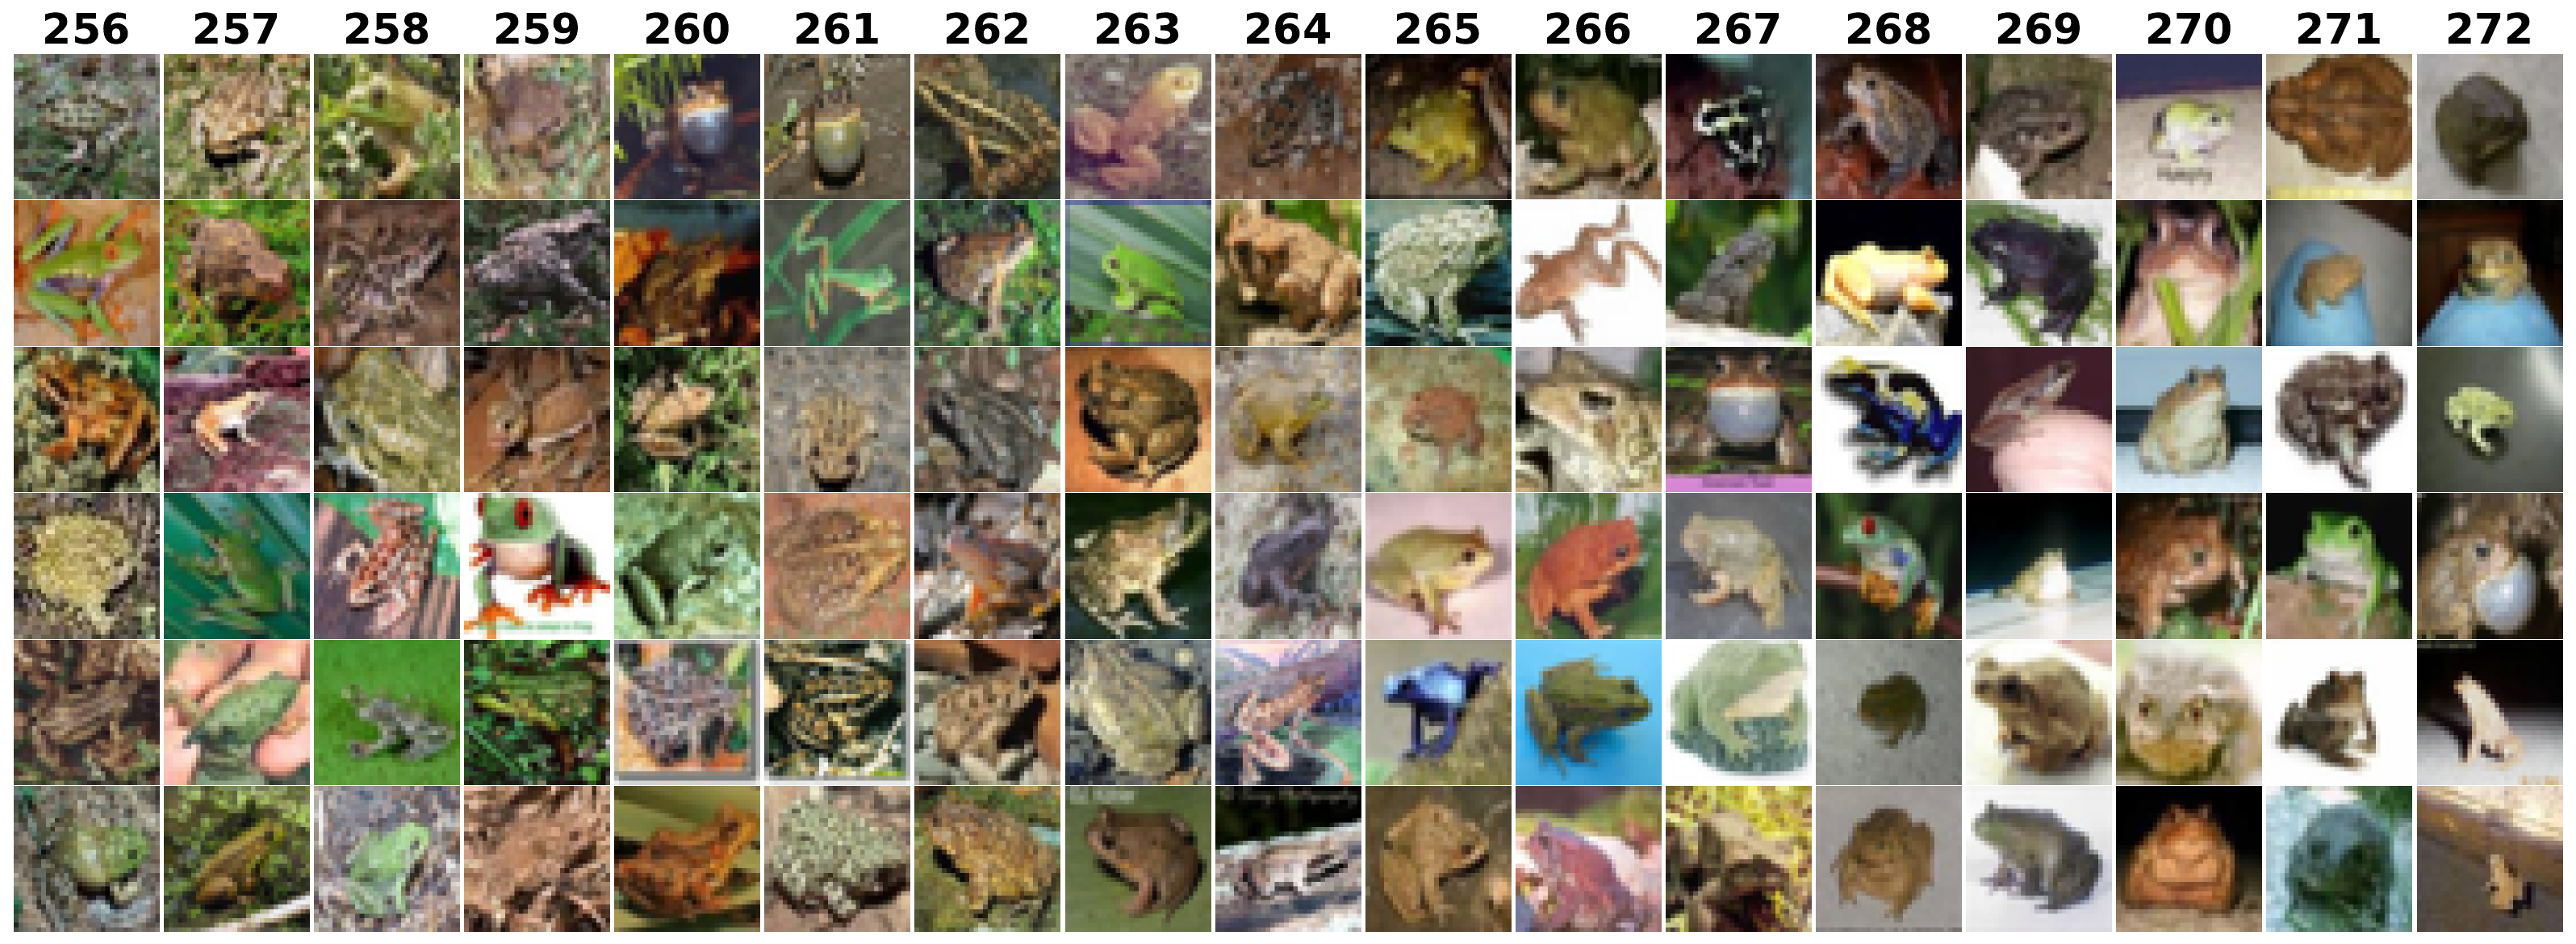}}
    \subfigure[bird]{\includegraphics[width=0.49\textwidth]{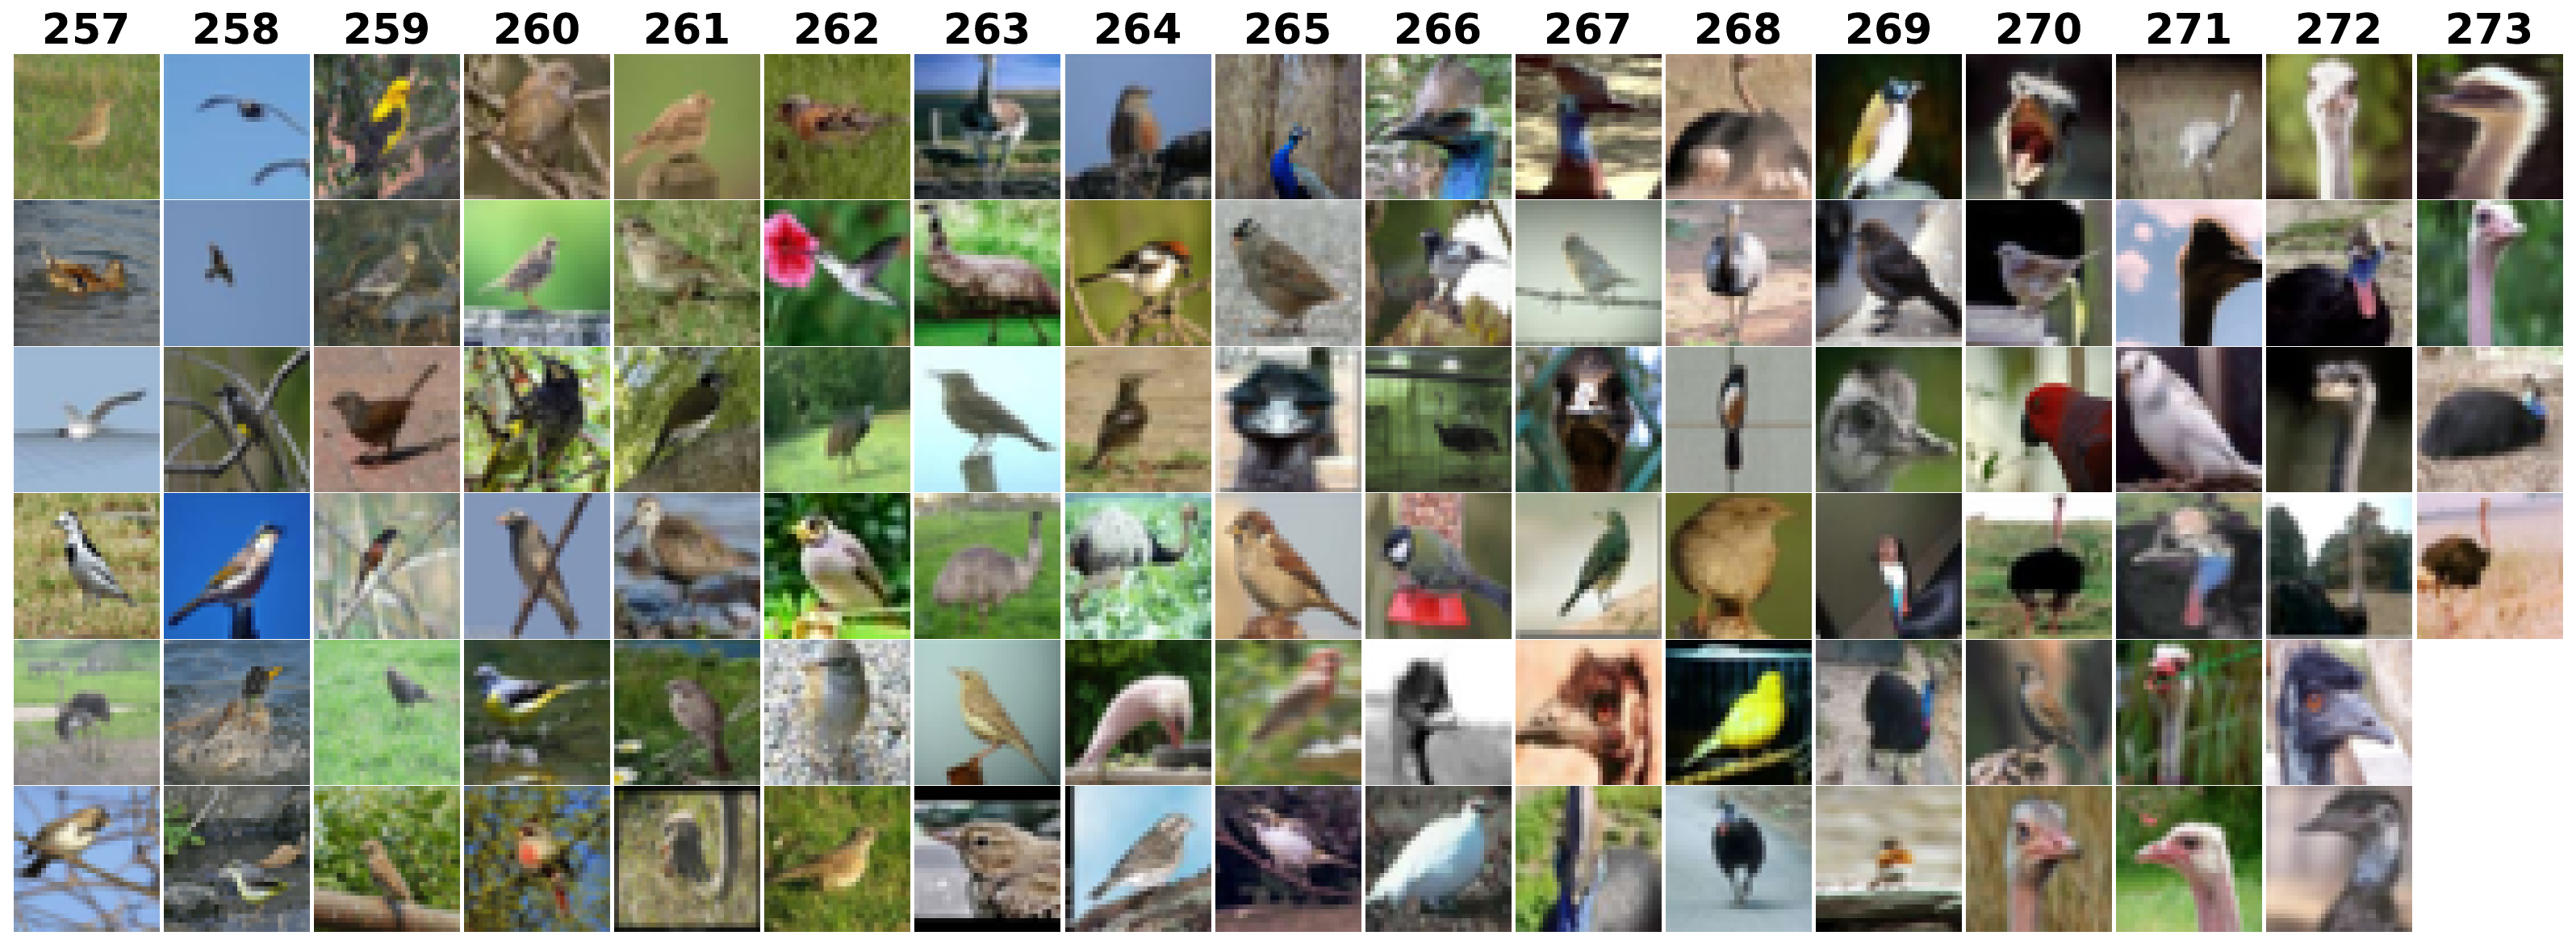}}
    \subfigure[ship]{\includegraphics[width=0.50\textwidth]{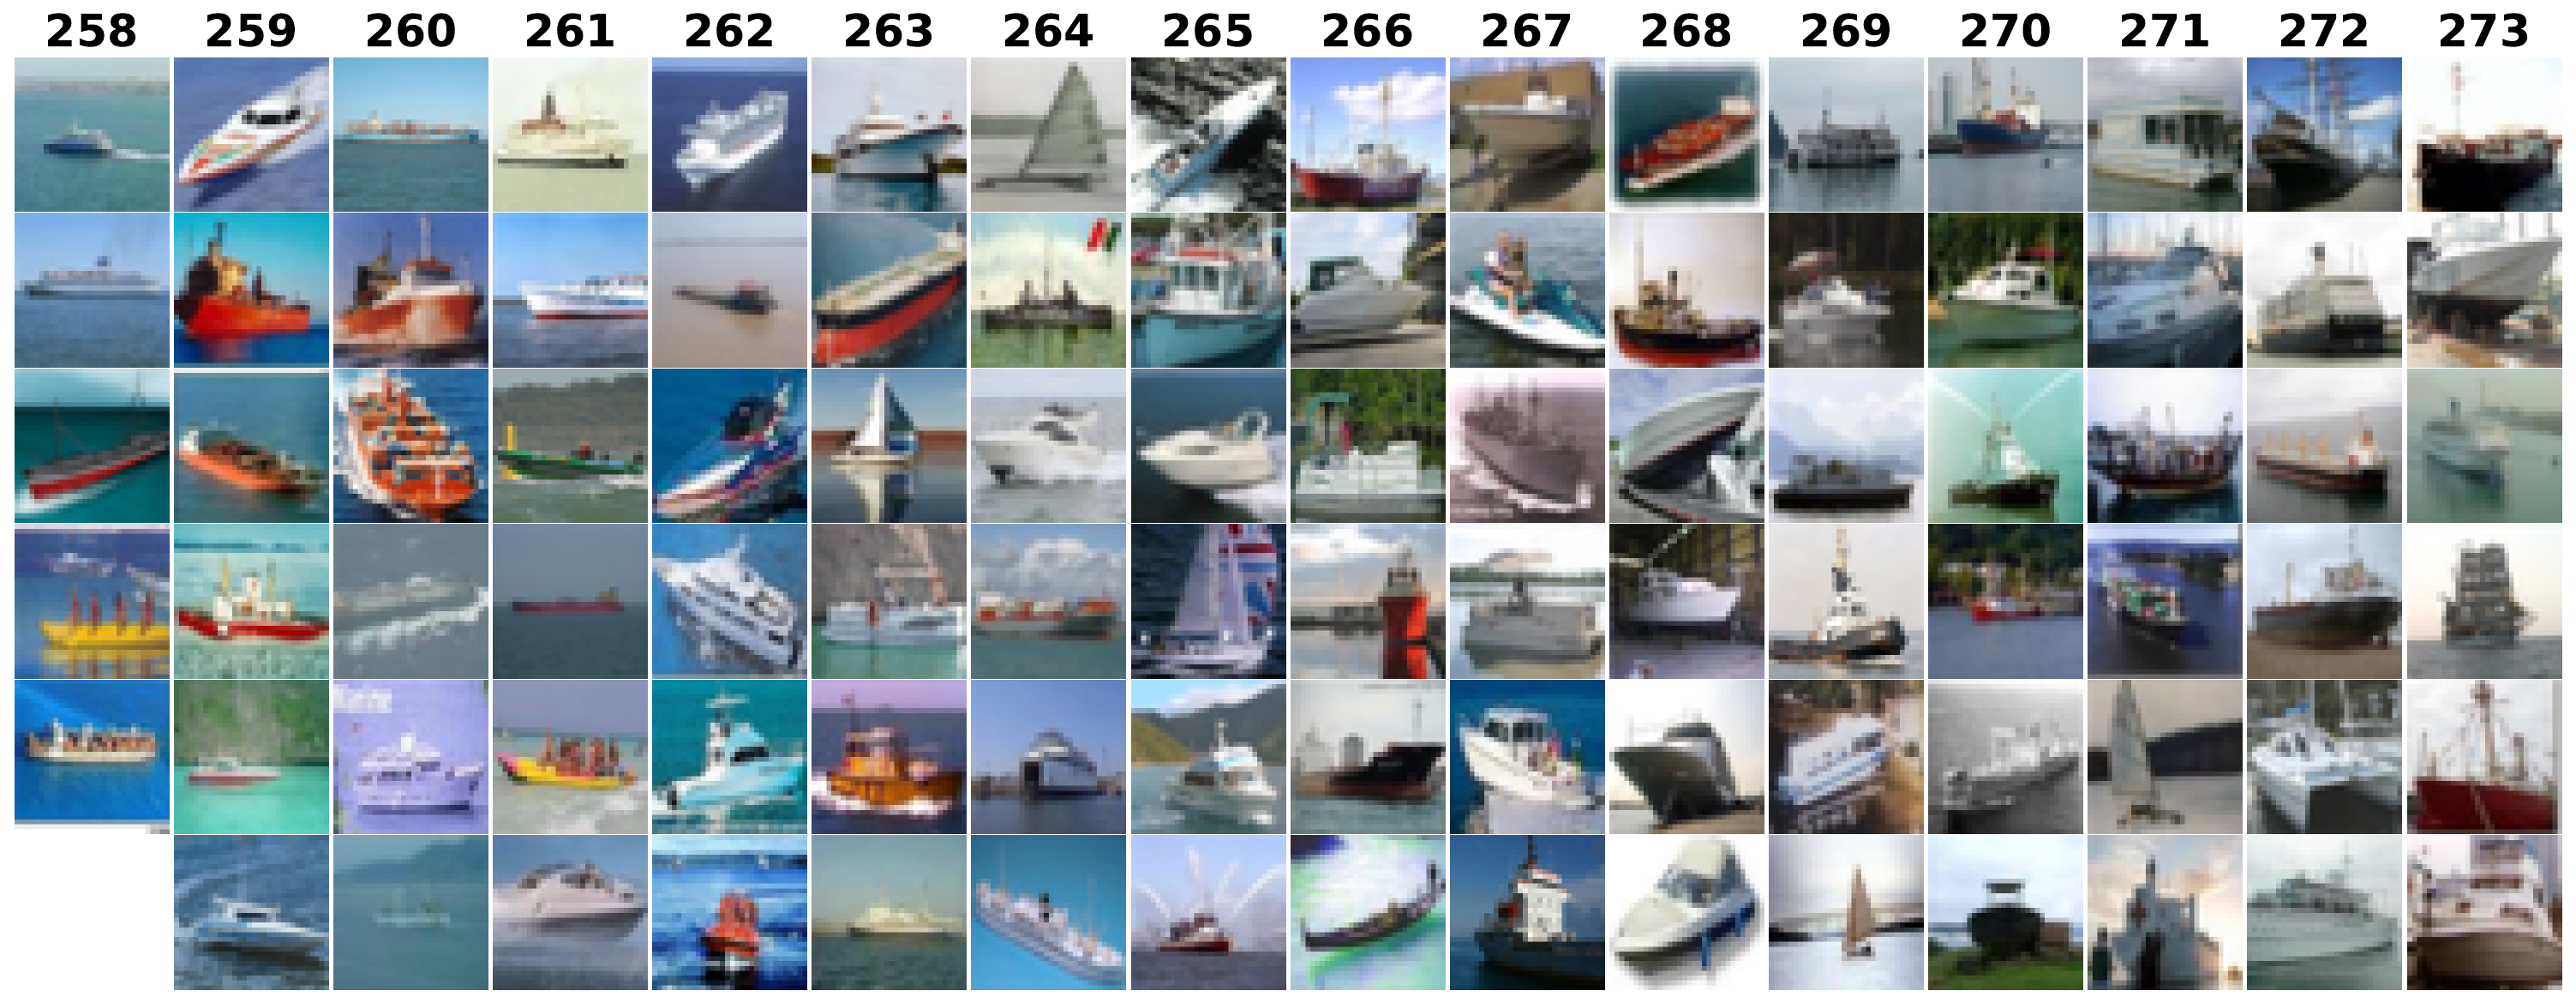}}
    \subfigure[airplane]{\includegraphics[width=0.48\textwidth]{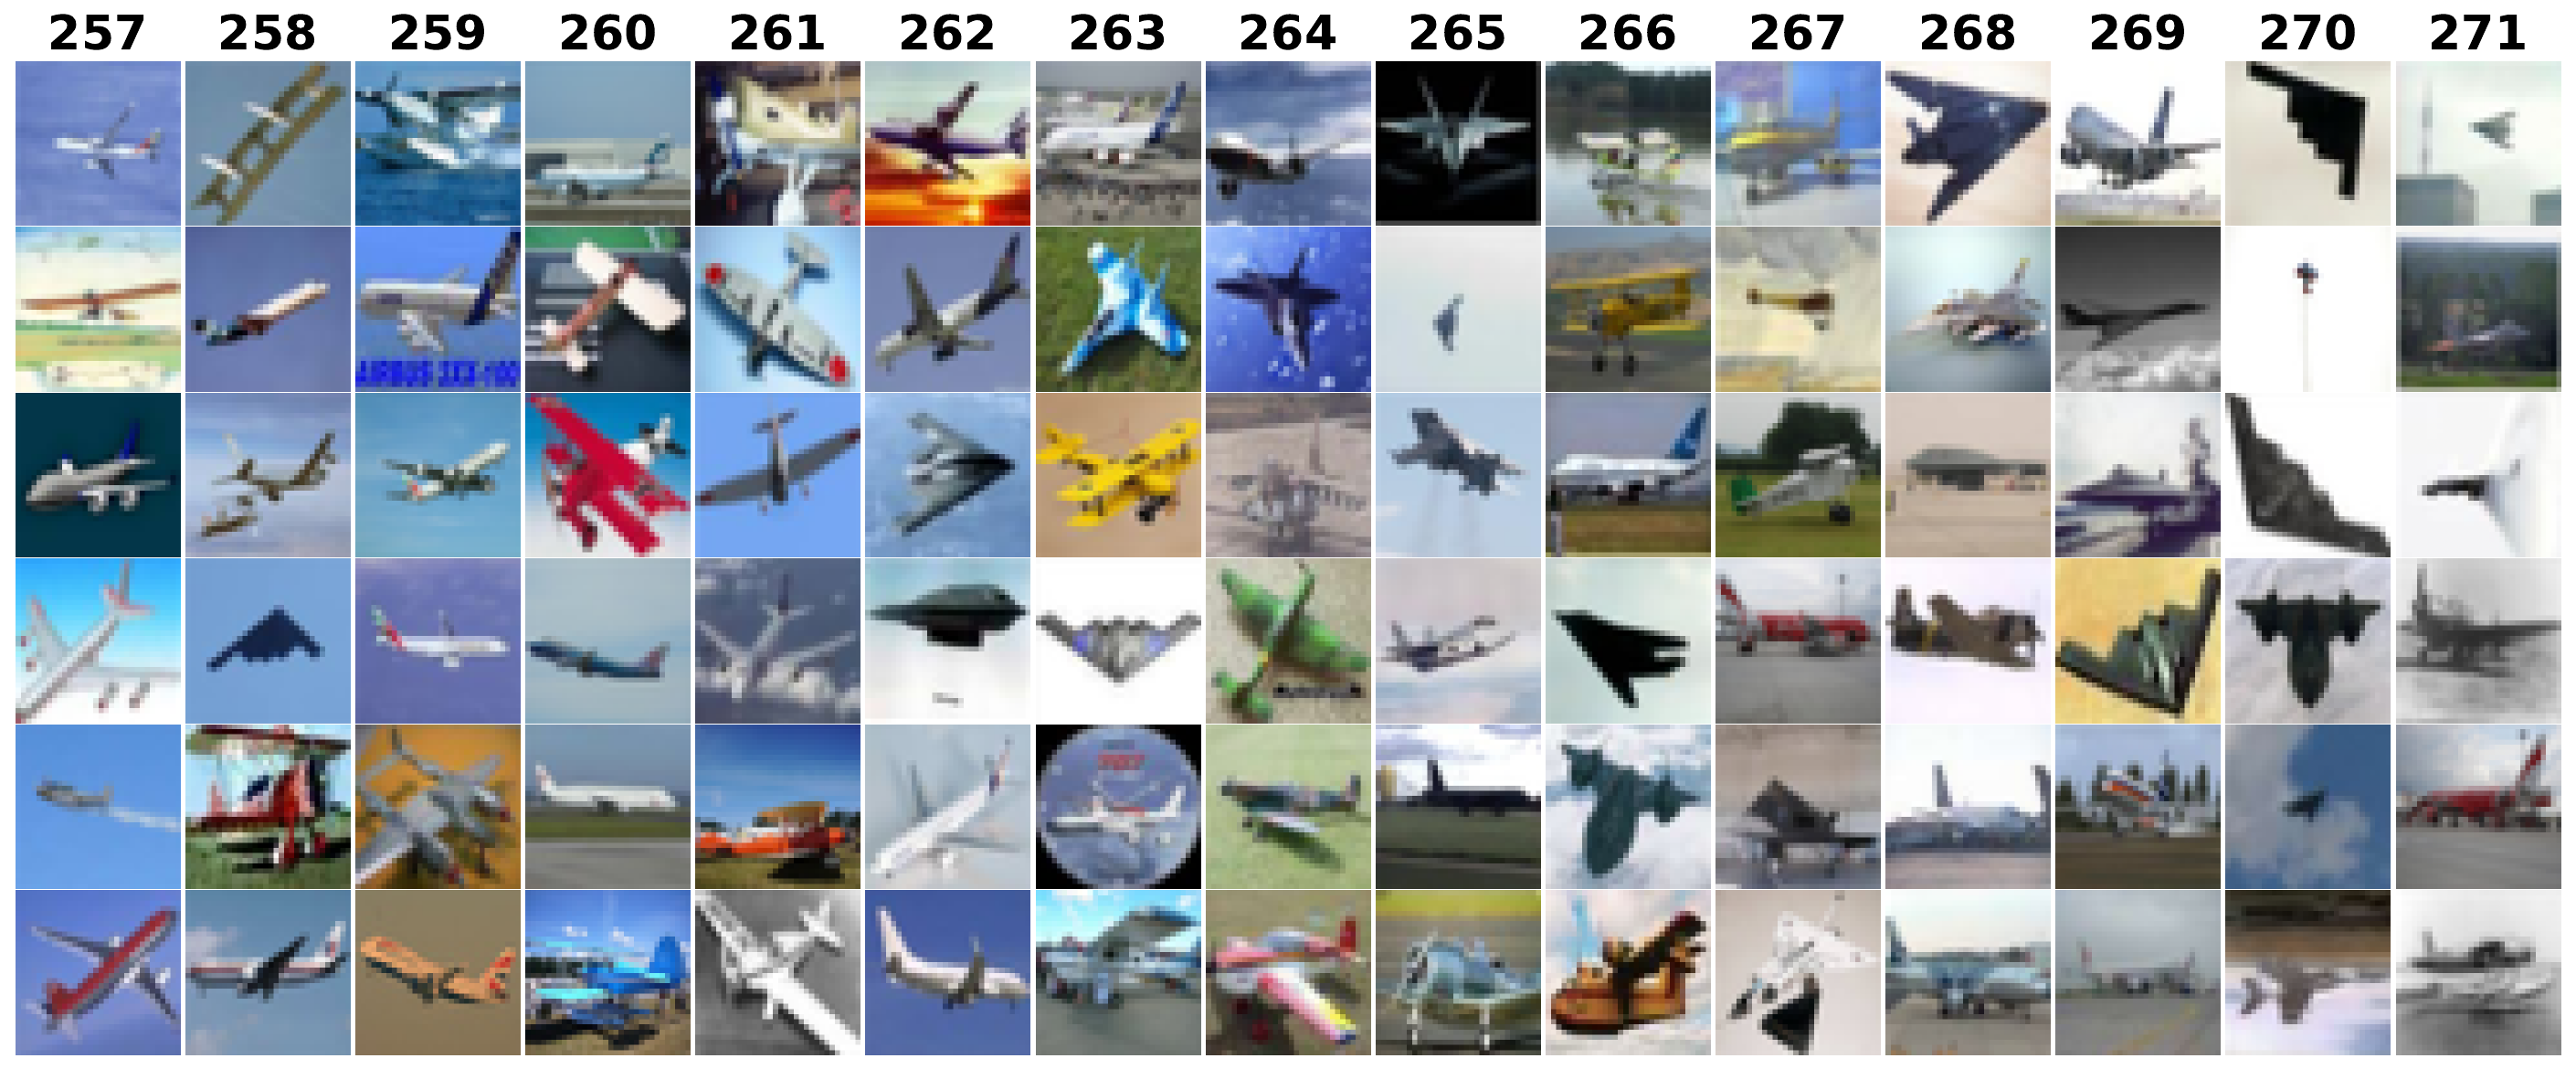}}
    \vspace{0.1cm}
    \caption{{\bf Image samples with corresponding NAIS-Net depth.} The
      figure shows samples from CIFAR-10 grouped by final network
      depth, for four different classes. The qualitative differences
      evident in images inducing different final depths indicate that
      NAIS-Net adapts processing systematically according
      characteristics of the data.  For example, \emph{``frog''}
      images with textured background are processed with fewer
      iterations than those with plain background. Similarly,
      \emph{``ship''} and \emph{``airplane''} images having a
      predominantly blue color are processed with lower depth than
      those that are grey/white, and \emph{``bird''} images are grouped
      roughly according to bird size with larger species such as
      ostriches and turkeys being classified with greater processing depth.}
    \label{fig:histdepth_sup}
\end{figure}
